# Supplementary material for: Feature Importance of Climate Vulnerability Indicators with Gradient Boosting across Five Global Cities
Source: arXiv:2411.10628 source file (2024-11-15)
Supplement: Supplementary file 1 [file appendix.tex]

\section{appendix} \label{sec:appendix}
The following pages include the survey instrument items that were analyzed for this study. 
The survey contained additional items that are being analyzed for a pre-registered study and being prepped for manuscript.
Please contact the authors for more information about the survey instrument.
[Consent]
Consent Form
Title of Research: Flood Disaster Policy Preferences
Principal Investigators: [redacted for peer review]
Research Institution: [redacted for peer review]
\vspace{5pt}

Key Information: Your informed consent is being sought for research. Participation in this research is voluntary. The purpose of the research is to better understand people's preferences with regard to possible policies that can help prepare for and recover from flood disasters. The expected duration of your participation is <15 minutes. You will be asked to complete a survey comparing various aspects of proposed policies related to flood disasters, as well as some additional demographic questions. There are no reasonably foreseeable risks or discomforts to you as a result of participation, and you may choose to end the survey at any time. Results from this survey will help to inform research and policymaking to prepare for and recover from flood disasters.
\vspace{5pt}

Confidentiality: All records from this study will be kept confidential. Your responses will be kept private, and we will not include any information that will make it possible to identify you in any report we might publish. Research records will be stored securely on password-protected computers. The research team will be the only party that will have access to your data.  
\vspace{5pt}

Compensation: You will be compensated according to your participant account type. Please refer to the invitation that you received to participate in this survey for further information about your compensation.
\vspace{5pt}

Contact Information for IRB (human subjects research): If you have questions regarding your rights as a research subject, or if problems arise which you do not feel you can discuss with the Principal Investigators, please contact the Institutional Review Board (IRB) at:
Phone: [redacted for peer review]
Email: [redacted for peer review]
\vspace{5pt}

Summary: I understand the information that was presented and that:
My participation is voluntary.
Refusal to participate will involve no penalty or loss of benefits to which I am otherwise entitled.
\vspace{5pt}

I may discontinue participation at any time without penalty or loss of benefits.
I do not waive any legal rights or release [redacted for peer review] or its agents from liability for negligence.
\vspace{5pt}

[consent] If you are at least 18 years old and would like to continue with this survey, please provide your consent below.
\vspace{5pt}

I am at least 18 years old and consent to participate in this survey (1)
\vspace{5pt}

I do not consent (0)
\vspace{5pt}

[VPN]
[VPSWarning]
Warning! 
This survey uses a protocol to check that you are responding from inside the U.S. and not using a Virtual Private Server (VPS), Virtual Private Network (VPN), or a proxy to hide your country. In order to take this survey, please turn off your VPS/VPN/proxy if you are using one and also any ad-blocking applications.
Failure to do this might prevent you from completing the survey.
[VPSDetect]
\vspace{5pt}

Our system has detected that you are using a Virtual Private Server (VPS) or proxy to mask your country location. As has been widely reported, this has caused a number of problems with survey data.
Because of this, we cannot let you participate in this study. If you are located in the U.S., please turn off your VPS the next time you participate in a survey, as we requested in the warning message at the beginning. If you are outside of the U.S., we apologize, but this study is directed only towards U.S. participants.
Thank you for your interest in our study.
\vspace{5pt}

[VPSNotUS]
Our system has detected that you are attempting to take this survey from a location outside of the U.S. Unfortunately, this study is only directed towards participants in the U.S. and we cannot accept responses from those in other countries.
Thank you for your interest in our study.
\vspace{5pt}

[VPSCountryNA]
For some reason, we were unable to verify your country location. By continuing, you are certifying that you are taking this survey from the U.S. and not using a VPS. We will be checking locations manually after the survey is complete and you might not receive payment if this check identifies you as violating these requirements.
\vspace{5pt}

I certify that I am taking the survey from the U.S. and am not using a VPS
\vspace{5pt}

I cannot certify the above
[Captcha]
\vspace{5pt}

Before you proceed to the survey, please complete the captcha below.
\vspace{5pt}

I’m not a robot
\vspace{5pt}

[Extreme Weather Experience]
[experience] Have you personally ever had significant experiences with extreme weather events or natural disasters? (1-5) 
(randomized)
\vspace{5pt}

(For each of the following extreme weather events, indicate how OFTEN a significant event has occurred for you in your lifetime.)
\vspace{5pt}

[rain] Flooding from heavy rainfall
\vspace{5pt}

[coast] Flooding from coastal storms
\vspace{5pt}

[river] Flooding from river overflows
\vspace{5pt}

[wind] Heavy winds 
\vspace{5pt}

[heat] Heatwaves / extreme heat
\vspace{5pt}

[drought] Droughts
\vspace{5pt}

[fire] Wildfires
\vspace{5pt}

[quake] Earthquakes 
\vspace{5pt}

Never (1) 
\vspace{5pt}

Rarely – has occurred for me once or twice in my life (2)
\vspace{5pt}

Sometimes – has occurred for me every 2-5 years (3)
\vspace{5pt}

Regularly – has typically occurred for me 1-2 times each year (4)
\vspace{5pt}

Frequently – has typically occurred for me 3+ times each year (5)
\vspace{5pt}

[Psychological Traits]
\vspace{5pt}

[self\_vul] How much more likely are you (or family members that you live with) to experience harm from flood disasters – as compared to other people living in NYC? (1-5)
\vspace{5pt}

Not at all likely to be harmed more (1)
\vspace{5pt}

Slightly likely to be harmed more (2)
\vspace{5pt}

Moderately likely to be harmed more (3)
\vspace{5pt}

Very likely to be harmed more (4)
\vspace{5pt}

Extremely likely to be harmed more (5)
\vspace{5pt}

[discrimination] In the past two weeks, how often do you feel that you have been treated unfairly because of your race/ethnicity, gender/sexuality, disability, or other identity? (1-5)
\vspace{5pt}

Not at all (1)
\vspace{5pt}

Slightly often (2)
\vspace{5pt}

Moderately often (3)
\vspace{5pt}

Very often (4)
\vspace{5pt}

Extremely often (5)
\vspace{5pt}

[Demographics]
\vspace{5pt}

[age] What year were you born?
\vspace{5pt}

[education] 
\vspace{5pt}

What is the highest level of education you have completed?
\vspace{5pt}

[none] No formal education (0)
\vspace{5pt}

[less\_hs] Less than a high school degree or G.E.D. (1)
\vspace{5pt}
[hs] High school degree or G.E.D. (2)
\vspace{5pt}
[associate] Associate’s degree or vocational degree (3)
\vspace{5pt}
[undergrad] Bachelor’s degree (4)
\vspace{5pt}
[grad] Graduate or professional degree (5)
\vspace{5pt}
[gender] What is your gender? (randomized)
\vspace{5pt}
Woman (1)
\vspace{5pt}
Man (2)
\vspace{5pt}
Non-binary (3)
\vspace{5pt}
Prefer to self-describe (4)
\vspace{5pt}

[queer] Do you consider yourself a member of the Queer / LGBTQ+ community? 
\vspace{5pt}
Yes (1)
\vspace{5pt}
No (0)
\vspace{5pt}

[disability] Do you consider yourself to have impaired mobility and/or another disability?
\vspace{5pt}
Yes (1)
\vspace{5pt}
No (0)

\vspace{5pt}
[income_USD] What was your total household income, before taxes, in 2023? 
This figure should include the total annual income, before taxes, of all of the members of your family living in your home. (USD)
\vspace{5pt}
(1) Less than USD10,000
\vspace{5pt}
(2) USD 10000 – USD19,999
\vspace{5pt}
(3) USD20,000 – USD29,999
\vspace{5pt}
(4) USD30,000 – USD39,999
\vspace{5pt}
(5) USD40,000 – USD49,999
\vspace{5pt}
(6) USD50,000 – USD59,999	
\vspace{5pt}
(7) USD60,000 – USD69,999 
\vspace{5pt}
(8) USD70,000 – USD79,999	 (median)
\vspace{5pt}
(9) USD80,000 – USD89,999
\vspace{5pt}
(10) USD90,000 – USD99,999
\vspace{5pt}
(11) USD100,000 – USD109,999
\vspace{5pt}
(12) USD110,000 – USD119,999
\vspace{5pt}
(13) USD120,000 – USD129,999
\vspace{5pt}
(14) USD130,000 – USD139,999
\vspace{5pt}
(15) USD140,000 – USD149,999
\vspace{5pt}
(16) USD150,000 – USD159,999
\vspace{5pt}
(17) More than USD160,000
\vspace{5pt}
\vspace{5pt}
[language] Do you primarily speak a language other than English at home or with your immediate family? 
\vspace{5pt}
Yes (1)
\vspace{5pt}
No (0)
